# Supplementary material for: User Retention-oriented Recommendation with Decision Transformer
Source: arXiv:2303.06347 source file (2023-03-11)
Supplement: Supplementary file 1 [file 10Appendix.tex]

\appendix

\section{Model-based User Retention Score}
\begin{figure}[h]
	\centering
	%	\hspace*{-7mm}1.049
	\includegraphics[width=1.02\linewidth]{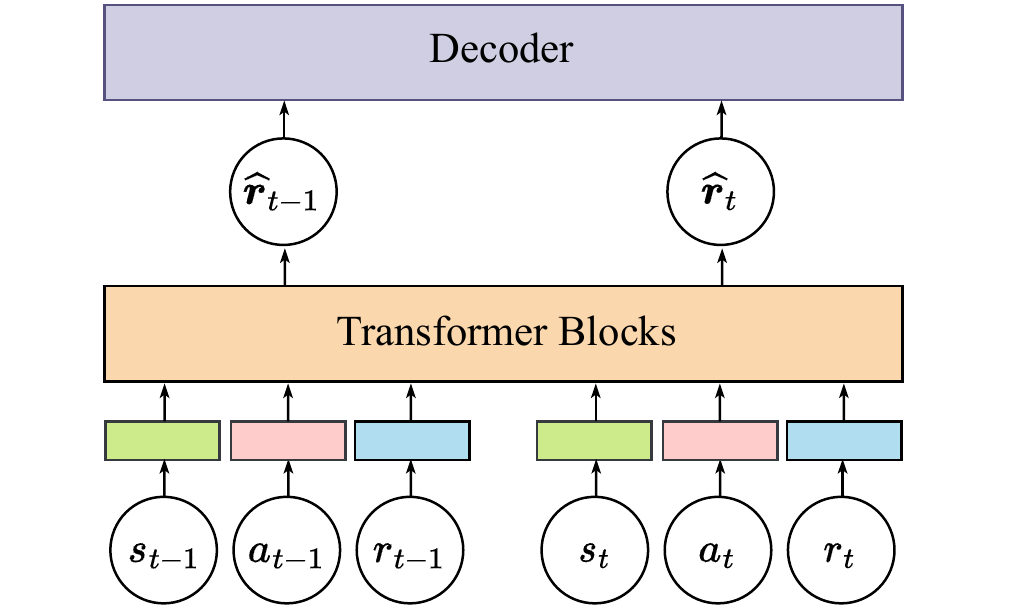}
	% \vspace*{-3mm}
	\caption{Framework of model-based user retention score.}
	\label{fig:model}
% 	\vspace*{-3mm}
\end{figure}

To illustrate our Model-based user retention score more clearly, we also show its structure in Figure \ref{fig:model}. We train a supervised model to predict the rewards according to the actions in the current states. We view DT's reconstruction of $a_t$ as a prediction of reward $r_t$, denoting it as $\widehat{\boldsymbol{r}}_{t}$. Then, we utilize a feed-forward neural layer as decoder to transform the embedding $\widehat{\boldsymbol{r}}_{t}$ into a value $\widetilde{r}_{t}$. Then, we can calculate the MSE loss.
We denote the output of our DT4Rec as $\overline{\boldsymbol{A}}=[\overline{\boldsymbol{a}}_{1},\ldots,\overline{\boldsymbol{a}}_{t},\ldots,\overline{\boldsymbol{a}}_{T}]$, where $\overline{\boldsymbol{a}}_{t}$ is the predicted item sequence at the t-th timestep.
When we evaluate our DT4Rec with the model-based user retention score, we form states, actions and rewards into sequences as: 
\begin{equation}\small
\widehat{\tau}=[s_{1}, \overline{\boldsymbol{a}}_{1}, r_{1}, \ldots, s_{t}, \overline{\boldsymbol{a}}_{t}, r_{t}, \ldots, s_{T}, \overline{\boldsymbol{a}}_{T}, r_{T},].
\end{equation}
Then we input the sequence $\widehat{\tau}$ into supervised model to predict the rewards according to the recommended item sequences in the current states.

\section{Hyperparameter Setting}
In this subsection, we introduce the hyperparameter setting of our baselines. In the prediction accuracy task, our baselines are BERT4Rec and SASRec, which are both Transformer-based models. For fair and convenient comparison, we set the Transformer layer number as 2, the head number as 8, embedding size as 128, which are the same as our models. For sequence length, we set it from [10, 20, 30, 40, 50]. We set the mask ratio of BERT4Rec from [0.1, 0.2, 0.3, 0.4, 0.5]. In the user retention task, we set the parameters as recommended by the authors for our baselines.
